# Supplementary material for: Discourse-Driven Evaluation: Unveiling Factual Inconsistency in Long Document Summarization
Source: arXiv:2502.06185 source file (2025-02-10)
Supplement: Supplementary file 1 [file appendix_aggrefact.tex]

\begin{table}[t!]
\scriptsize
\centering
\begin{NiceTabular}{lcc|r}
 \toprule
& \textbf{\textsc{AggreFact-}} & \textbf{\textsc{AggreFact-}}\\
& \textbf{\textsc{Cnn-FtSota}} & \textbf{\textsc{Xsum-FtSota}} & \textsc{Avg}\\
\midrule
\RowStyle{\color{gray}}
 DAE    & 65.4 ± 3.6 & 70.2 ± 1.8 & 67.8\\
 \RowStyle{\color{gray}}
 \textsc{QuestEval}    &70.2 ± 3.0 & 59.6 ± 1.9 & 64.9\\
 \RowStyle{\color{gray}}
\textsc{Summac-ZS}    &    64.0 ± 3.2 & 56.4 ± 1.4 & 60.2\\
\RowStyle{\color{gray}}
\textsc{SummaC-CV}      &61.0 ± 3.1 & 65.0 ± 2.0 & 63.0\\
\RowStyle{\color{gray}}
 \textsc{QAFactEval}     &  67.8 ± 3.9 &  63.9 ± 2.0 & 65.9\\
      
     % \textsc{AlignScore}       & 62.5 ± 3.1  &  69.6 ± 1.8\\
% \RowStyle{\color{gray}}
 \textsc{AMRFact}\textsuperscript{{$\diamond$}} & 72.3 ± 2.5 & 64.1 ± 1.8 &  68.2 \\
  \textsc{Fizz} & 72.6 ± 3.0 &69.3 ± 1.9  & 71.0 \\
\midrule
\RowStyle{\color{gray}}
\textsc{ChatGPT-ZS} & 56.3 ± 2.9 & 62.7 ± 1.7 & 59.5 \\
\RowStyle{\color{gray}}
\textsc{ChatGPT-COT}&  52.5 ± 3.3 &  55.9 ± 2.1 & 54.2\\
\RowStyle{\color{gray}}
\textsc{ChatGPT-DA}& 53.7 ± 3.5 & 54.9 ± 1.9 & 54.3  \\
\RowStyle{\color{gray}}
\textsc{ChatGPT-Star} & 56.3 ± 3.1&  57.8 ± 0.2  & 57.1\\
G-EVAL\textsuperscript{$\diamond$} & 69.9 ± 3.5 & 65.8 ± 1.9 & 67.9\\
\midrule 
  \textsc{AlignScore}       & 62.5 ± 3.1  &  69.6 ± 1.8 & 66.1\\
\textsc{StructS}-level1 & 64.7 ± 3.1 & 69.1 ± 1.9 & 66.9 \\
\textsc{StructS}-level2 & 64.6 ± 2.9 &  \textbf{70.4} ± 1.9 & 67.5\\
\textsc{StructS}-level3 & 65.0 ± 2.8 & 66.5 ± 1.9 & 65.8\\

\midrule
\end{NiceTabular}
\caption{ Balanced binary accuracy using a single threshold on the \textsc{AggreFact-FtSota}  subset (single-threshold setting). We show 95\% confidence intervals. \textcolor{gray}{Gray colored}  results are taken from \cite{tang-etal-2023-understanding} and \textsuperscript{$\diamond$} results are taken from \cite{qiu2023amrfact}.}\label{tab:aggrefact_blacc_resul}
\end{table}
